# Supplementary material for: Back-Translated Task Adaptive Pretraining: Improving Accuracy and Robustness on Text Classification
Source: arXiv:2107.10474 source file (2021-07-22)
Supplement: Supplementary file 1 [file appendix.tex]

\clearpage

\appendix

\section{Examples}

As supplement materials, we provide some examples of back translated sentence which used in further re-training (\textbf{BT-TAPT}) in Table \ref{tab:bt-examples} and the noisy examples used in the robustness experiment in Table \ref{tab:noise-examples}.

\begin{table*}
\centering
\small
\resizebox{\textwidth}{!}{
\begin{tabular}{>{\raggedright}p{9cm}p{9cm}}
\toprule 
\textbf{Original Sentences}  & \textbf{Back Translated Sentences}\\
\midrule 
This movie is AWFUL! I don't even know where to begin, I'm speechless I can't even describe how awful this is. The blood is flourescent first of all, and the acting is AWFUL! The only good part was the biker chick that saves the day. This movie was rediculous, I don't see how it could even get a vote of 1 its so bad. It looks like it was made by highschool students. & I don't even know where to start, I'm speechless, I can't put into words how terrible it is, the blood is beginning to drip and the acting is disgusting. Just good thing it was the biker chick Callum who'd been cut off on the bike wall. This film wasn't venerable, I don't know how he managed to get it to top of 1. It feels like it was made by the high richtung students. \\
\midrule
As much as I like Japanese movies this one didn't just cut it... A movie that is supposed to be about rebels and the survival of a royal blood line turned out to be a very slow paced movie with a doubtful plot.The photography is OK, though I've seen much better sword fight scenes in other Japanese movies, the fast cameras and the way they followed the characters didn't convince me at all. The soundtrack is so weak you don't even notice its presence.But worst of all was the way the plot evolved.I have to admit that, at some times, I had a hard time understanding who was who and what was going on...Anyway the platonic love between the main character and another one was completely unnecessary and seemed to come from a Hollywood influence.All in all, if your looking for an action Japanese movie this isn't it. Its very slow, with very few sword fight scenes and very sentimental... in a bad way… & As much as I like Japanese films, a film doesn't take it easy. A film that would be about rebellion and the survival of a royal bloodline turned out to be a very slow and dubious doom and gloom. The shots are fine although I have always seen much bigger sword fighting scenes before from other Japanese movies, but the high speed cameras and the way they followed the characters haven't convinced me. The soundtrack is so weak it hardly recognizes its presence, but the most serious thing is the development of the storyline. I must admit that I sometimes had difficulty in understanding who was who and what. In any event, the platonic love between the main character and another guy was wholly unnecessary, and seemed written off by Hollywood influences. Now, start you bet on a Japanese action film with only a few sword-fight scenes and a rather bitter sensation... \\
\midrule
Such a delightful movie! Very heart warming. One can't help falling in love with the character of Gigi. He's adorable as a child and grows into a sensitive artist. The whole movie revolves around him. He lives in a wonderful world living all life curiosity, desire and anticipation. There is an elder brother who tries to steal his glory but really remains in the shadow all his life. The father is very stereotypically Italian and so is the mother. I wanted the father to come and reunite with the mother in the last scene and have them cry and laugh. I also wish that there was at least something redeeming about the elder brother. His personality seems to have been trashed entirely. Passion and ardour that's the key to life. And looking through the camera focusing on small details and savoring the delicate details of life & A Wonderful Film! Very heartwarming, suddenly you're falling in love with the character of Gigi, who is just like someone who became both an incredible artist and a fine singer and very special puppet. The entire movie revolves around Christ who lives in a wonderful world and who experiences all phases of life over a lifetime: Curiosity, longing and anticipation. The older sibling tries to steal his fame, but stays largely in the shadows throughout his life, with his father - just like his mother - being shaped by stereotypes of an Italian lifestyle. In the last scene, I wanted father and mother who we reencounter to cry, and laugh, and also the older brother a little bit redemption. His personality seems to be totally destroyed; passion and schendahl - that's the key to life autos, and staring through a camera, Topper concentrates on the small details of his tools and relishes the finer details of life \\
\midrule
I honestly want the last 30 minuets of my life back.The only person that is fit to watch this movie is Helen Keller I kept saying to myself this has to get better this has to get better.Then the zombies finally showed up and they had some raccoon paint on there eyes.They talked like regular people.One drove a car.Some voodoo woman asked what one of the \"Zombies\" wanted and the \" zombie\" said ( I want to Dance)( THAT WAS IT) Out came the movie I couldn't take it any longer Can I sue for a \u00bd hour of my life????? & I honestly want to get versions of the last 30 minutes of my life back, Helen Keller... Helen Keller is the only person who is fit to see this film and I kept telling myself that when things get better you don't take the trouble. Then finally came the zombies and had raccoon paint on their eyes. We gave each other a talk. One drove their car.... Some women asked me where any of the \"zombies\" was hiding and he did not answer (THAT it was): That was why the film finished I can no longer take it for dyce? A dangerous business? \\
\bottomrule
\end{tabular}}
\caption{Back translated examples of IMDB reviews.}
\label{tab:bt-examples}
\end{table*}

\begin{table*}
\centering
\small
 \resizebox{\textwidth}{!}{
\begin{tabular}{p{1.5cm}p{15cm}}
\toprule 
\textbf{Original Sentence}& Prediction Unit Helps Forecast Wildfires (AP). AP - It's barely dawn when Mike Fitzpatrick starts his shift with a blur of colorful maps, figures and endless charts, but already he knows what the day will bring. Lightning will strike in places he expects. Winds will pick up, moist places will dry and flames will roar.\\
\midrule[0.03em]
\textbf{Synonym}& Prediction Unit service Forecast Wildfires (AP). AP - It's barely dayspring when Mike Fitzpatrick starts his shift with a blur of colorful maps figures and endless charts but already he knows what the day will bring. Lightning will strike in invest he expects. farting will pick up moist stead will dry and flames will roar.\\
\midrule[0.03em]
\textbf{BT Beam}& Prediction Unit helps forecast wildfires (AP) AP - No sooner does it dawn than Mike Fitzpatrick begins his shift with a blur of colorful maps, numbers, and endless charts than he knows what the day will bring. Lightning will strike places it expects, winds will flare up, damp places will dry up and flames will flare up.\\
\midrule[0.03em]
\textbf{BT top-p}& Prediction Unit (AP) helps forecast wildfires AP - Tune out, Mike Fitzpatrick starts his shift and puffs up colorful maps, numbers and endless charts. Occasionally lightning will strike, breezes will zip in places, drying moist places and flames will burst.\\
\midrule[0.03em]
\textbf{Char Swap}& Prediction Unit Helps Forecast Wildfires (AP). AQ - It's barely dawn when iMke Fitzpatrick starts his shift with a blur of colorful maps figures and endless charts but already he knows what the day will Qring. Lightning will strike in places he exNects. Winds will pick up moist places will drIy and flames will roar.\\
\midrule[0.03em]
\textbf{InvTest}& Prediction Unit Helps Forecast Wildfires (AP). AP - It's barely dawn when Deen Vuong starts his shift with a blur of colorful maps figures and endless charts but already he knows what the day will bring. Lightning will strike in places he expects. Winds will pick up moist places will dry and flames will roar.\\

\bottomrule
\end{tabular}}
% }
\caption{Example of the original sentence of \textsc{AGNews} and five different types of noisy sentences.} 
\label{tab:noise-examples}
\end{table*}

\begin{table*}
\centering
\small
 \resizebox{\textwidth}{!}{
\begin{tabular}{p{1.5cm}p{15cm}}
\toprule 
\textbf{Original Sentence}& those who managed to avoid the deconstructionist theorizing of french philosopher jacques derrida in college can now take an 85 minute brush up course with the documentary derrida .\\
\midrule[0.03em]
\textbf{Synonym}& those who managed to avoid the deconstructionist theorizing of french philosopher jacques derrida in college can now make an 85 infinitesimal brush up course with the documentary derrida .\\
\midrule[0.03em]
\textbf{BT Beam}& Those who managed to escape French philosopher Jacques Derrida's deconstructivist theory formation in college can now take an 85-minute refresher course with the documentary film derrida.\\
\midrule[0.03em]
\textbf{BT top-p}& Those who escaped French philosopher Jacques Derrida'gies de Derrida's de-practical theories at a college will be able to attend an 85-minute re-examination course.\\
\midrule[0.03em]
\textbf{Char Swap}& those who managed to avoid the deconstructionist theorizing of french philsopher jacques derrida in Yollege can now take an 85 minute brush up course with the documentary derrida .\\
\midrule[0.03em]
\textbf{InvTest}& those who managed to avoid the deconstructionist theorizing of french philosopher jacques Hulett in college can now take an 130 minute brush up course with the documentary derrida.\\

\bottomrule
\end{tabular}}
% }
\caption{Example of the original sentence of \textsc{SST2} and five different types of noisy sentences.} 
\label{tab:noise-examples}
\end{table*}
