# Supplementary material for: Back-Translated Task Adaptive Pretraining: Improving Accuracy and Robustness on Text Classification
Source: arXiv:2107.10474 source file (2021-07-22)
Supplement: Supplementary file 3 [file appendix_noise_sample_ag.tex]

\begin{table*}
\centering
\small
 \resizebox{\textwidth}{!}{
\begin{tabular}{p{1.5cm}p{15cm}}
\toprule 
\textbf{Original Sentence}& Prediction Unit Helps Forecast Wildfires (AP). AP - It's barely dawn when Mike Fitzpatrick starts his shift with a blur of colorful maps, figures and endless charts, but already he knows what the day will bring. Lightning will strike in places he expects. Winds will pick up, moist places will dry and flames will roar.\\
\midrule[0.03em]
\textbf{Synonym}& Prediction Unit service Forecast Wildfires (AP). AP - It's barely dayspring when Mike Fitzpatrick starts his shift with a blur of colorful maps figures and endless charts but already he knows what the day will bring. Lightning will strike in invest he expects. farting will pick up moist stead will dry and flames will roar.\\
\midrule[0.03em]
\textbf{BT Beam}& Prediction Unit helps forecast wildfires (AP) AP - No sooner does it dawn than Mike Fitzpatrick begins his shift with a blur of colorful maps, numbers, and endless charts than he knows what the day will bring. Lightning will strike places it expects, winds will flare up, damp places will dry up and flames will flare up.\\
\midrule[0.03em]
\textbf{BT top-p}& Prediction Unit (AP) helps forecast wildfires AP - Tune out, Mike Fitzpatrick starts his shift and puffs up colorful maps, numbers and endless charts. Occasionally lightning will strike, breezes will zip in places, drying moist places and flames will burst.\\
\midrule[0.03em]
\textbf{Char Swap}& Prediction Unit Helps Forecast Wildfires (AP). AQ - It's barely dawn when iMke Fitzpatrick starts his shift with a blur of colorful maps figures and endless charts but already he knows what the day will Qring. Lightning will strike in places he exNects. Winds will pick up moist places will drIy and flames will roar.\\
\midrule[0.03em]
\textbf{InvTest}& Prediction Unit Helps Forecast Wildfires (AP). AP - It's barely dawn when Deen Vuong starts his shift with a blur of colorful maps figures and endless charts but already he knows what the day will bring. Lightning will strike in places he expects. Winds will pick up moist places will dry and flames will roar.\\

\bottomrule
\end{tabular}}
% }
\caption{Example of the original sentence of \textsc{AGNews} and five different types of noisy sentences.} 
\label{tab:noise-examples}
\end{table*}
