# Supplementary material for: Back-Translated Task Adaptive Pretraining: Improving Accuracy and Robustness on Text Classification
Source: arXiv:2107.10474 source file (2021-07-22)
Supplement: Supplementary file 4 [file appendix_noise_sample_sst2.tex]

\begin{table*}
\centering
\small
 \resizebox{\textwidth}{!}{
\begin{tabular}{p{1.5cm}p{15cm}}
\toprule 
\textbf{Original Sentence}& those who managed to avoid the deconstructionist theorizing of french philosopher jacques derrida in college can now take an 85 minute brush up course with the documentary derrida .\\
\midrule[0.03em]
\textbf{Synonym}& those who managed to avoid the deconstructionist theorizing of french philosopher jacques derrida in college can now make an 85 infinitesimal brush up course with the documentary derrida .\\
\midrule[0.03em]
\textbf{BT Beam}& Those who managed to escape French philosopher Jacques Derrida's deconstructivist theory formation in college can now take an 85-minute refresher course with the documentary film derrida.\\
\midrule[0.03em]
\textbf{BT top-p}& Those who escaped French philosopher Jacques Derrida'gies de Derrida's de-practical theories at a college will be able to attend an 85-minute re-examination course.\\
\midrule[0.03em]
\textbf{Char Swap}& those who managed to avoid the deconstructionist theorizing of french philsopher jacques derrida in Yollege can now take an 85 minute brush up course with the documentary derrida .\\
\midrule[0.03em]
\textbf{InvTest}& those who managed to avoid the deconstructionist theorizing of french philosopher jacques Hulett in college can now take an 130 minute brush up course with the documentary derrida.\\

\bottomrule
\end{tabular}}
% }
\caption{Example of the original sentence of \textsc{SST2} and five different types of noisy sentences.} 
\label{tab:noise-examples}
\end{table*}
